# Supplementary material for: Dynamic Vaccine Prioritization via Non-Markovian Final-state Optimization
Source: arXiv:2511.07200 source file (2025-11-10)
Supplement: Supplementary file 1 [file si.pdf]

# Supplementary Information for

## Dynamic Vaccine Prioritization via Non-Markovian Final-state Optimization

Mi Feng[1,4], Liang Tian*[1,3], Changsong Zhou†[1,2,3]

[1]Department of Physics, Hong Kong Baptist University, Kowloon Tong, Hong Kong SAR 999077, China
[2]Centre for Nonlinear Studies and Beijing-Hong Kong-Singapore Joint Centre for Nonlinear and Complex Systems (Hong Kong), Hong Kong Baptist University, Kowloon Tong, Hong Kong SAR 999077, China
[3]Institute of Computational and Theoretical Studies, Hong Kong Baptist University, Kowloon, Hong Kong SAR 999077, China
[4]Institute for Research and Continuing Education, Hong Kong Baptist University, Shenzhen, Guangdong, 518057, China

# Supplementary Note 1 State Aggregation

In this section, we show how to (i) derive the parameters of a general model from those of a detailed model, and (ii) recover the time evolution of each state in the detailed model from simulations of the general model.

As in Fig. 1d of the main text, once an individual becomes infected, their infection course is partitioned into four states: exposed, asymptomatic, presymptomatic, and symptomatic. For each state we define a hazard for generating infections and a hazard for exiting the state. Specifically, we use $\omega_{\text{inf}}^{\text{exp}}(\tau)$, $\omega_{\text{inf}}^{\text{asym}}(\tau)$, $\omega_{\text{inf}}^{\text{presym}}(\tau)$, $\omega_{\text{inf}}^{\text{sym}}(\tau)$ and $\omega_{\text{exit}}^{\text{exp}}(\tau)$, $\omega_{\text{exit}}^{\text{asym}}(\tau)$, $\omega_{\text{exit}}^{\text{presym}}(\tau)$, $\omega_{\text{exit}}^{\text{sym}}(\tau)$. Individuals in the exposed state are not infectious, so $\omega_{\text{inf}}^{\text{exp}}(\tau) \equiv 0$. In the general model, "exit from the infected state" coincides with removal; at the level of detailed states we keep the subscript "exit" (not "rem") to avoid confusion.

Following the Methods in the main text, we also introduce the associated survival functions $\Psi_{\text{inf}}^{\text{exp}}(\tau)$, $\Psi_{\text{inf}}^{\text{asym}}(\tau)$, $\Psi_{\text{inf}}^{\text{presym}}(\tau)$, $\Psi_{\text{inf}}^{\text{sym}}(\tau)$ and $\Psi_{\text{exit}}^{\text{exp}}(\tau)$, $\Psi_{\text{exit}}^{\text{asym}}(\tau)$, $\Psi_{\text{exit}}^{\text{presym}}(\tau)$, $\Psi_{\text{exit}}^{\text{sym}}(\tau)$, with event–time densities $\psi_{\text{inf}}^{\text{exp}}(\tau)$, $\psi_{\text{inf}}^{\text{asym}}(\tau)$, $\psi_{\text{inf}}^{\text{presym}}(\tau)$, $\psi_{\text{inf}}^{\text{sym}}(\tau)$ and $\psi_{\text{exit}}^{\text{exp}}(\tau)$, $\psi_{\text{exit}}^{\text{asym}}(\tau)$, $\psi_{\text{exit}}^{\text{presym}}(\tau)$, $\psi_{\text{exit}}^{\text{sym}}(\tau)$.

The instantaneous ability to generate infections within a state is governed jointly by the infection and exit processes and can be written as $\Omega(\tau) = \omega_{\text{inf}}(\tau)\Psi_{\text{exit}}(\tau)$. By adding superscripts we obtain $\Omega^{\text{exp}}(\tau)$, $\Omega^{\text{asym}}(\tau)$, $\Omega^{\text{presym}}(\tau)$, $\Omega^{\text{sym}}(\tau)$. In the general model (with a single infected and a single removed class), $\Omega(\tau)$ is the generation–time density, denoted $\psi_{\text{gen}}(\tau)$. Intuitively, $\Omega(\tau)$ is the probability density of producing an infection at state age $\tau$, where the factor $\Psi_{\text{exit}}(\tau)$ enforces that the individual has not exited that state before $\tau$.

We first aggregate the presymptomatic and symptomatic phases. If we view "presym + sym" as one block, the distribution of the time to exit that block is the convolution of the exit–time distributions of its two components:

$$\psi_{\text{exit}}^{\text{presym+sym}} = \psi_{\text{exit}}^{\text{presym}} * \psi_{\text{exit}}^{\text{sym}}, \tag{S1.1}$$

where $*$ denotes convolution.

Next, upon leaving the exposed state, an individual enters the asymptomatic block with probability $\varrho_{\text{asym}}$ and the presymptomatic–symptomatic block with probability $\varrho_{\text{presym}} = 1 - \varrho_{\text{asym}}$. The exit–time distribution from the "post-exposed" block is therefore

$$\psi_{\text{exit}}^{\text{presym+sym+asym}} = (1 - \varrho_{\text{asym}}), \psi_{\text{exit}}^{\text{presym+sym}} + \varrho_{\text{asym}}, \psi_{\text{exit}}^{\text{asym}}. \tag{S1.2}$$

*liangtian@hkbu.edu.hk
†cszhou@hkbu.edu.hk

Finally, the overall removal (from infection) time density is

$$\psi_{\text{rem}} = \psi_{\text{exit}}^{\text{exp}} * [(1-\varrho_{\text{asym}})\psi_{\text{exit}}^{\text{presym}} * \psi_{\text{exit}}^{\text{sym}} + \varrho_{\text{asym}}\psi_{\text{exit}}^{\text{asym}}] \,. \tag{S1.3}$$

The corresponding survival and hazard functions are $\Psi_{\text{rem}}(\tau) = 1 - \int_0^\tau \psi_{\text{rem}}(\tau')d\tau'$ and $\omega_{\text{rem}}(\tau) = \psi_{\text{rem}}(\tau)/\Psi_{\text{rem}}(\tau)$.

At the level of infection generation, presymptomatic and symptomatic phases combine as

$$\Omega^{\text{presym+sym}} = \Omega^{\text{presym}} + \psi_{\text{exit}}^{\text{presym}} * \Omega^{\text{sym}}. \tag{S1.4}$$

The first term accounts for transmissions that occur while still presymptomatic; the second term accounts for transmissions after leaving presymptomatic at some state time $\tau'$ (distributed as $\psi_{\text{exit}}^{\text{presym}}$) and then spending $\tau - \tau'$ time in the symptomatic phase. Then, mixing with the asymptomatic branch gives

$$\Omega^{\text{presym+sym+asym}} = (1-\varrho_{\text{asym}}), \Omega^{\text{presym+sym}} + \varrho_{\text{asym}}, \Omega^{\text{asym}}. \tag{S1.5}$$

Since exposed individuals are non-infectious, the overall generation–time density (the infection kernel for the general model) is obtained by convolving the exit from exposed with the post-exposed infection kernel:

$$\psi_{\text{gen}} = \Omega = \psi_{\text{exit}}^{\text{exp}} * [\varrho_{\text{asym}}\Omega^{\text{asym}} + (1-\varrho_{\text{asym}})\left(\Omega^{\text{presym}} + \psi_{\text{exit}}^{\text{presym}} * \Omega^{\text{sym}}\right)] \,. \tag{S1.6}$$

Given $\psi_{\text{gen}}$ and $\Psi_{\text{rem}}$, the infection hazard in the general model satisfies $\omega_{\text{inf}}(\tau) = \psi_{\text{gen}}(\tau)/\Psi_{\text{rem}}(\tau)$. And we can obtain the survival function and infection time distribution as $\Psi_{\text{inf}}(\tau) = \exp\left(-\int_0^\tau \omega_{\text{inf}}(\tau')d\tau'\right)$ and $\psi_{\text{inf}}(\tau) = \omega_{\text{inf}}(\tau)\Psi_{\text{inf}}(\tau)$.

Additionally, because asymptomatic infections do not result in death, the age stratified infection fatality rates (IFRs) in the general model are calculated by: $\boldsymbol{\epsilon} = (1-\varrho_{\text{asym}}), \boldsymbol{\epsilon}_{\text{sym}}$.

Let $\boldsymbol{i}_\bullet(t)$ the fractions currently in state $\bullet$. Individuals infected at time $t'$ remain exposed at time $t$ with probability $\Psi_{\text{exit}}^{\text{exp}}(t-t')$, hence

$$\boldsymbol{i}_{\text{exp}}(t) = \int_0^t \Psi_{\text{exit}}^{\text{exp}}(t-t')d\boldsymbol{c}(t'). \tag{S1.7}$$

The flux leaving exposed is $d\left(\boldsymbol{c}(t) - \boldsymbol{i}_{\text{exp}}(t)\right)$, and weight the post-exposed inflow by $\varrho_{\text{asym}}$ and survival in asymptomatic:

$$\boldsymbol{i}_{\text{asym}}(t) = \varrho_{\text{asym}} \int_0^t \Psi_{\text{exit}}^{\text{asym}}(t-t')d\left(\boldsymbol{c}(t') - \boldsymbol{i}_{\text{exp}}(t')\right). \tag{S1.8}$$

Analogously,

$$\boldsymbol{i}_{\text{presym}}(t) = (1-\varrho_{\text{asym}}) \int_0^t \Psi_{\text{exit}}^{\text{presym}}(t-t')d\left(\boldsymbol{c}(t') - \boldsymbol{i}\text{exp}(t')\right). \tag{S1.9}$$

The inflow to symptomatic at time $t'$ equals the outflow from presymptomatic, which can be expressed as $d\left[(1-\varrho_{\text{asym}})\left(\boldsymbol{c}(t') - \boldsymbol{i}_{\text{exp}}(t')\right) - \boldsymbol{i}_{\text{presym}}(t')\right]$. Convolving with survival in the symptomatic state yields

$$\boldsymbol{i}_{\text{sym}}(t) = \int_0^t \Psi_{\text{exit}}^{\text{sym}}(t-t')d\left[(1-\varrho_{\text{asym}})\left(\boldsymbol{c}(t') - \boldsymbol{i}_{\text{exp}}(t')\right) - \boldsymbol{i}_{\text{presym}}(t')\right]. \tag{S1.10}$$

# Supplementary Note 2 Analysis of Final-state Equivalence

Because Eqs. 1–2 in the main text exactly reproduce the corresponding Monte Carlo simulations: we consider a large population whose age distribution is $\boldsymbol{\rho}$; contact probabilities between age groups are governed by the contact matrix $\boldsymbol{A}$ together with a global scaling factor $k$; for an infected individual with infection age in $[\tau, \tau + d\tau)$, the probability of delivering a transmission is $\omega_{\text{inf}}(\tau)d\tau$, and the probability of

removal is $\omega_{\text{rem}}(\tau)d\tau$. By standard results, its final state can be predicted directly from the initial state via the Kermack–McKendrick final-size relation, which is usually used in the Markovian framework:

$$\tilde{\boldsymbol{c}} = \mathbf{1} - \boldsymbol{s}(0) \odot \exp\left(-k\lambda_{\text{eff}}\mathbf{A}\,\text{diag}\left(\boldsymbol{\rho}\right)\left(\tilde{\boldsymbol{c}} - \tilde{\boldsymbol{r}}(0)\right)\right) \tag{S2.11}$$

where $\lambda_{\text{eff}} = \int_0^\infty \omega_{\text{inf}}(\tau)\exp\left(-\int_0^\tau \omega_{\text{rem}}(\tau')d\tau'\right)d\tau$.

To forecast the final state from an arbitrary time $t$, we treat $t$ as a new initial time and regard all currently infected individuals as new infection seeds. These seeds have infection ages $t - t'$, where $t'$ is each individual's infection time (individuals infected after time $t$ begin with infection age 0 as usual). The residual effective infection rate for a seed of age $t - t'$ is $\lambda_\dagger = \int_{t-t'}^\infty \omega_{\text{inf}}(\tau)\exp\left(-\int_{t-t'}^\tau \omega_{\text{rem}}(\tau')d\tau'\right)d\tau$.

We note that $\lambda_{\text{eff}}$ represents the total infection capacity of infected individual from his/her infection. When predicting from time $t$, we must subtract the infection capacity already "used up" by the seeds, namely $\lambda_{\text{eff}} - \lambda_\dagger$.

To do this, we need the distribution (by age group) of seed infection ages at time $t$, obtainable from infection history via the removal survival $\Psi_{\text{rem}}$: the mass of seeds infected at $t'$ and still not removed at $t$ is $\Psi_{\text{rem}}(t - t')d\boldsymbol{c}(t')$. Hence, $\lambda_{\text{eff}}\left(\tilde{\boldsymbol{c}} - \tilde{\boldsymbol{r}}(0)\right)$ should be subtracted by:

$$\int_0^t \left(\lambda_{\text{eff}} - \int_{t-t'}^\infty \omega_{\text{inf}}(\tau)\exp\left(-\int_{t-t'}^\tau \omega_{\text{rem}}(\tau')d\tau'\right)d\tau\right)\Psi_{\text{rem}}(t-t')d\boldsymbol{c}(t') \tag{S2.12}$$

$$= \int_0^t \left(\lambda_{\text{eff}} - \int_{t-t'}^\infty \omega_{\text{inf}}(\tau)\Psi_{\text{rem}}(\tau)d\tau/\Psi_{\text{rem}}(t-t')\right)\Psi_{\text{rem}}(t-t')d\boldsymbol{c}(t') \tag{S2.13}$$

$$= \lambda_{\text{eff}}\boldsymbol{i}(t) - \int_0^t \int_{t-t'}^\infty \omega_{\text{inf}}(\tau)\Psi_{\text{rem}}(\tau)d\tau d\boldsymbol{c}(t') \tag{S2.14}$$

Define $\widehat{\boldsymbol{\lambda}}_{\text{eff}}(t) := \lambda_{\text{eff}} - \int_0^t \int_{t-t'}^\infty \omega_{\text{inf}}(\tau)\Psi_{\text{rem}}(\tau)d\tau d\boldsymbol{c}(t') \oslash \boldsymbol{i}(t)$, then the mid-epidemic final-size relation then becomes

$$\tilde{\boldsymbol{c}} = \mathbf{1} - \boldsymbol{s}(0) \odot \exp\left(-k\mathbf{A}\,\text{diag}\left(\boldsymbol{\rho}\right)\left(\lambda_{\text{eff}}\tilde{\boldsymbol{c}} - \lambda_{\text{eff}}\tilde{\boldsymbol{r}}(0) - \widehat{\boldsymbol{\lambda}}_{\text{eff}}(t) \odot \boldsymbol{i}(t)\right)\right) \tag{S2.15}$$

# Supplementary Note 3 Simulation with Lookahead Sliding Window

To clarify how the lookahead sliding window operates, we provide pseudocode for our SIRP simulator as shown in Algorithm 1. The core idea is to maintain a $\delta$-day future cache. At initialization we compute and store the trajectory over $(0, \delta]$, which forms the initial lookahead window. We denote the right edge of this window by $t^*$ and the current time by $t$ (initially, $t = 0$ and $t^* = \delta$). To advance one step, we (i) compute the new slice at $t^* + \Delta t$ and append it to the right of the window, (ii) commit the next cached slice at $t + \Delta t$ to the main time series, and (iii) set $t \leftarrow t + \Delta t$ and $t^* \leftarrow t^* + \Delta t$. This push-right/pop-left procedure keeps the window length fixed at $\delta$ while moving the simulation forward by $\Delta t$ each step.

When a vaccination is administered at time $t$, we immediately debit from the cached susceptibles at the maturity time $t + \delta$: $\boldsymbol{s}_{t^*} \leftarrow \boldsymbol{s}_{t^*} - \eta\boldsymbol{\vartheta}_t \odot (\boldsymbol{s}_{t^*} - \boldsymbol{u}_{t^*}) \oslash (\boldsymbol{s}_t - \boldsymbol{u}_t - \boldsymbol{v}_t)$ $\boldsymbol{s}_{t^*} - \boldsymbol{u}_{t^*}) \oslash (\boldsymbol{s}_t - \boldsymbol{u}_t - \boldsymbol{v}_t$ is the probability that a newly vaccinated susceptible remains uninfected throughout $(t, t + \delta]$. Because the window always exposes the post-vaccination state at $t + \delta$, we can immediately evaluate the final state after a vaccination at time $t$ without re-simulating the interval $(t, t + \delta]$, enabling fast optimization.

**Algorithm 1:** Simulation of non-Markovian SIRP epidemic dynamics with lookahead sliding window

**Input:** Contact coefficient $k$; contact matrix $\boldsymbol{A}$; population distribution $\boldsymbol{\rho}$; infection hazard $\omega_{\text{inf}}(\tau)$; removal hazard $\omega_{\text{rem}}(\tau)$; infection fatality rates (IFRs) $\boldsymbol{\epsilon}$; remaining life expectancy $\boldsymbol{\phi}$; vaccine response lag $\delta$; vaccine efficacy $\eta$; initial seeds $\boldsymbol{i}_{\text{seed}}$; horizon $T$, step $\Delta t$.

**Output:** Time series $\{\boldsymbol{s}_t, \boldsymbol{i}_t, \boldsymbol{r}_t, \boldsymbol{p}_t, \boldsymbol{v}_t, \boldsymbol{u}_t, \boldsymbol{c}_t, \boldsymbol{w}_t, \boldsymbol{d}_t, \boldsymbol{y}_t\}_{t=0}^{T}$

**Precompute:** $\Psi_{\text{inf}}(\tau) = \exp\big(-\int_0^\tau \omega_{\text{inf}}(\tau')\, d\tau'\big)$; $\Psi_{\text{rem}}(\tau) = \exp\big(-\int_0^\tau \omega_{\text{rem}}(\tau')\, d\tau'\big)$.

**Init:** $\boldsymbol{s}_0 \leftarrow \boldsymbol{1} - \boldsymbol{i}_{\text{seed}}$; $\boldsymbol{i}_0 \leftarrow \boldsymbol{i}_{\text{seed}}$; $\boldsymbol{r}_0, \boldsymbol{p}_0, \boldsymbol{v}_0, \boldsymbol{u}_0, \boldsymbol{w}_0, \boldsymbol{d}_0, \boldsymbol{y}_0 \leftarrow \boldsymbol{0}$; $\boldsymbol{c}_0 \leftarrow \boldsymbol{i}_{\text{seed}}$; $\Delta\boldsymbol{c}_0 \leftarrow \boldsymbol{c}_0$; $t \leftarrow 0$; $t^* \leftarrow 0$.

```
// Extend the right edge of the lookahead buffer from t* to t* + Δt
Function Lookahead():
    // Discrete kernel (generation time distribution) form survival functions
```
$\psi^{\text{gen}}_\tau \leftarrow (1 - \Psi_{\text{inf}}(\tau + \Delta t)/\Psi_{\text{inf}}(\tau))\, \Psi_{\text{rem}}(\tau)$;

```
    // Infectious pressure
```
$\boldsymbol{j}_{t^*} \leftarrow \boldsymbol{1} - \exp\Big(k\,\boldsymbol{A} \cdot \text{diag}\,(\boldsymbol{\rho}) \cdot \log\Big(\boldsymbol{1} - \sum_{t'=0}^{t^*} \psi^{\text{gen}}_{t'} \Delta\boldsymbol{c}_{t^*-t'}\Big)\Big)$;

```
    // New infections
```
$\Delta\boldsymbol{c}_{t^*+\Delta t} \leftarrow \boldsymbol{s}_{t^*} \odot \boldsymbol{j}_{t^*}$; $\boldsymbol{s}_{t^*+\Delta t} \leftarrow \boldsymbol{s}_{t^*} - \Delta\boldsymbol{c}_{t^*+\Delta t}$; $\boldsymbol{c}_{t^*+\Delta t} \leftarrow \boldsymbol{c}_{t^*} + \Delta\boldsymbol{c}_{t^*+\Delta t}$;

$\boldsymbol{u}_{t^*+\Delta t} \leftarrow \boldsymbol{u}_{t^*} - \boldsymbol{u}_{t^*} \odot \boldsymbol{j}(t^*)$;

```
    // Prevalent infected and removed (non-Markovian via survival)
```
$\boldsymbol{i}_{t^*+\Delta t} \leftarrow \sum_{t'=0}^{t^*+\Delta t} \Psi_{\text{rem}}(t^* - t')\, \Delta\boldsymbol{c}_{t'}$; $\boldsymbol{r}_{t^*+\Delta t} \leftarrow \sum_{t'=0}^{t^*+\Delta t} (1 - \Psi_{\text{rem}}(t^* - t'))\, \Delta\boldsymbol{c}_{t'}$;

```
    // Prevalent recovered, dead, and YLL
```
$\boldsymbol{w}_{t^*+\Delta t} \leftarrow (\boldsymbol{1} - \boldsymbol{\epsilon}) \odot \boldsymbol{r}_{t^*+\Delta t}$; $\boldsymbol{d}_{t^*+\Delta t} \leftarrow \boldsymbol{\epsilon} \odot \boldsymbol{r}_{t^*+\Delta t}$; $\boldsymbol{y}_{t^*+\Delta t} \leftarrow \boldsymbol{\epsilon} \odot \boldsymbol{r}_{t^*+\Delta t} \odot \boldsymbol{\phi}$);

```
// Prewarm: fill the lookahead buffer up to t* = δ
```
**while** $t^* < \delta$ **do**

  Lookahead(); $t^* \leftarrow t^* + \Delta t$

```
// Main loop: consume the left edge (t → t + Δt) and keep the buffer length δ
```
**while** $t < T$ **do**

```
    // Vaccination at time t and protection matures at t* = t + δ (optional)
```
  **if** VACCINATE *with* $\boldsymbol{\vartheta}_t$ **then**

    $\boldsymbol{\vartheta}_{\text{uninf}} \leftarrow \boldsymbol{\vartheta}_t \odot (\boldsymbol{s}_{t^*} - \boldsymbol{u}_{t^*}) \oslash (\boldsymbol{s}_t - \boldsymbol{u}_t - \boldsymbol{v}_t)$;

    $\boldsymbol{p}_{t^*} \leftarrow \boldsymbol{p}_{t^*} + \eta\boldsymbol{\vartheta}_{\text{uninf}}$; $\boldsymbol{u}_{t^*} \leftarrow \boldsymbol{u}_{t^*} + (1-\eta)\boldsymbol{\vartheta}_{\text{uninf}}$; $\boldsymbol{s}_{t^*} \leftarrow \boldsymbol{s}_{t^*} - \eta\boldsymbol{\vartheta}_{\text{uninf}}$;

    $\boldsymbol{v}_t \leftarrow \boldsymbol{v}_t + \boldsymbol{\vartheta}_t$;

```
    // Simulate one step
    Lookahead();
```
  $\boldsymbol{p}_{t^*+\Delta t} \leftarrow \boldsymbol{p}_{t^*}$; $\boldsymbol{v}_{t+\Delta t} \leftarrow \boldsymbol{v}_t - \boldsymbol{v}_t \odot \boldsymbol{j}(t)$;

  $t \leftarrow t + \Delta t$; $t^* \leftarrow t^* + \Delta t$

**return** $\{\boldsymbol{s}_t, \boldsymbol{i}_t, \boldsymbol{r}_t, \boldsymbol{p}_t, \boldsymbol{c}_t, \boldsymbol{w}_t, \boldsymbol{d}_t, \boldsymbol{y}_t\}_{t=0}^{T}$

# Supplementary Note 4 Robustness of Dynamic Vaccine Prioritization

To assess the robustness of our time-varying optimal vaccination strategy, specifically, its ability to retain superior performance across a wide range of epidemiological and logistical conditions, we additionally evaluate its effectiveness under variations in anther three key parameters: vaccination campaign duration ($T_{\text{vac}}$), daily vaccine rollout rate ($\theta$), and vaccine efficacy ($\eta$). Here, $T_{\text{vac}}$ specifies the total duration of the vaccine rollout; $\theta$ represents the daily vaccination capacity as a percentage of the population; and $\eta$

captures the efficacy of the vaccine in inducing protective immunity.

Figs. S1b–d show that empirical strategies retain predictable performance rankings across variations in $T_{\text{vac}}$, $\theta$, and $\eta$, but fail to improve adaptively across parameter changes. As expected, higher daily rollout rates ($\theta$) and longer campaign durations ($T_{\text{vac}}$) lead to better overall epidemic outcomes, with reductions in cumulative infections, deaths, and YLL across all strategies. In contrast, reductions in vaccine efficacy ($\eta$) diminish the effectiveness of all interventions. Notably, in every tested scenario, our FS-DVP consistently achieves the lowest final-state cumulative infections, deaths, and YLL, demonstrating its robustness and adaptability across a broad spectrum of plausible real-world conditions.

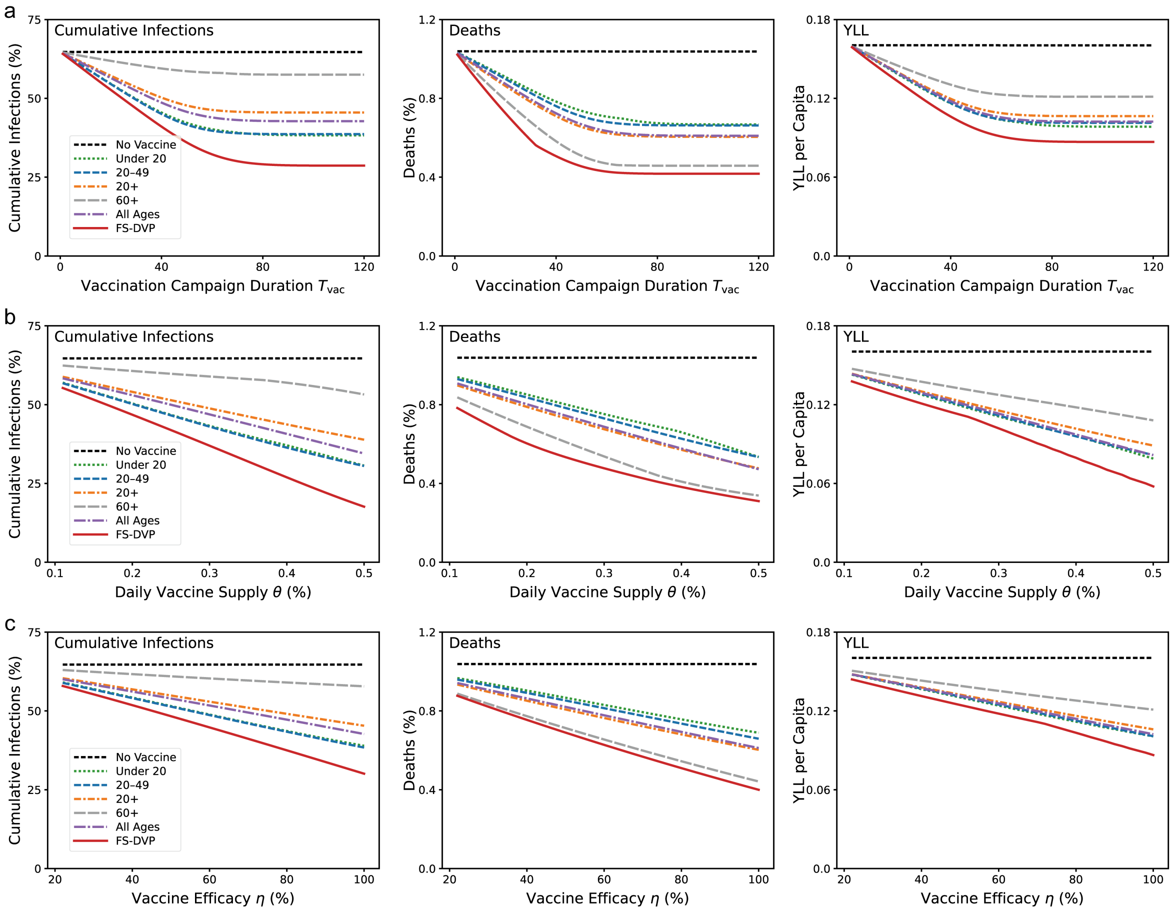


**Figure S1:** **a** Final-state cumulative infections, deaths, and years of life lost (YLL) across vaccination strategies under different vaccination campaign durations ($T_{\text{vac}}$). **b** Final-state outcomes under varying vaccine rollout rates ($\theta$). **c** Final-state outcomes under varying levels of vaccine efcacy ($\eta$).

# Supplementary Note 5 Mechanistic Insights of the Dynamic Optimal Vaccine Prioritization

NF-DVP is not universally optimal. There exist scenarios, especially for specific objectives or at intermediate transmission levels, where TS-DVP can perform slightly better. As shown in Fig. S2a, when the vaccination campaign lasts 60 days, there are parameter regions in which NF-DVP is not uniformly optimal. In particular, within a narrow moderate range of transmissibility ($R_0 \in [1.98, , 2.36]$), TS-DVP can temporarily outperform NF-DVP for reducing YLL.

A key reason is the intrinsic property of the receding-horizon control used by FS-DVP. At each vaccination decision time, the optimizer solves a final-state minimization problem that is optimal for that

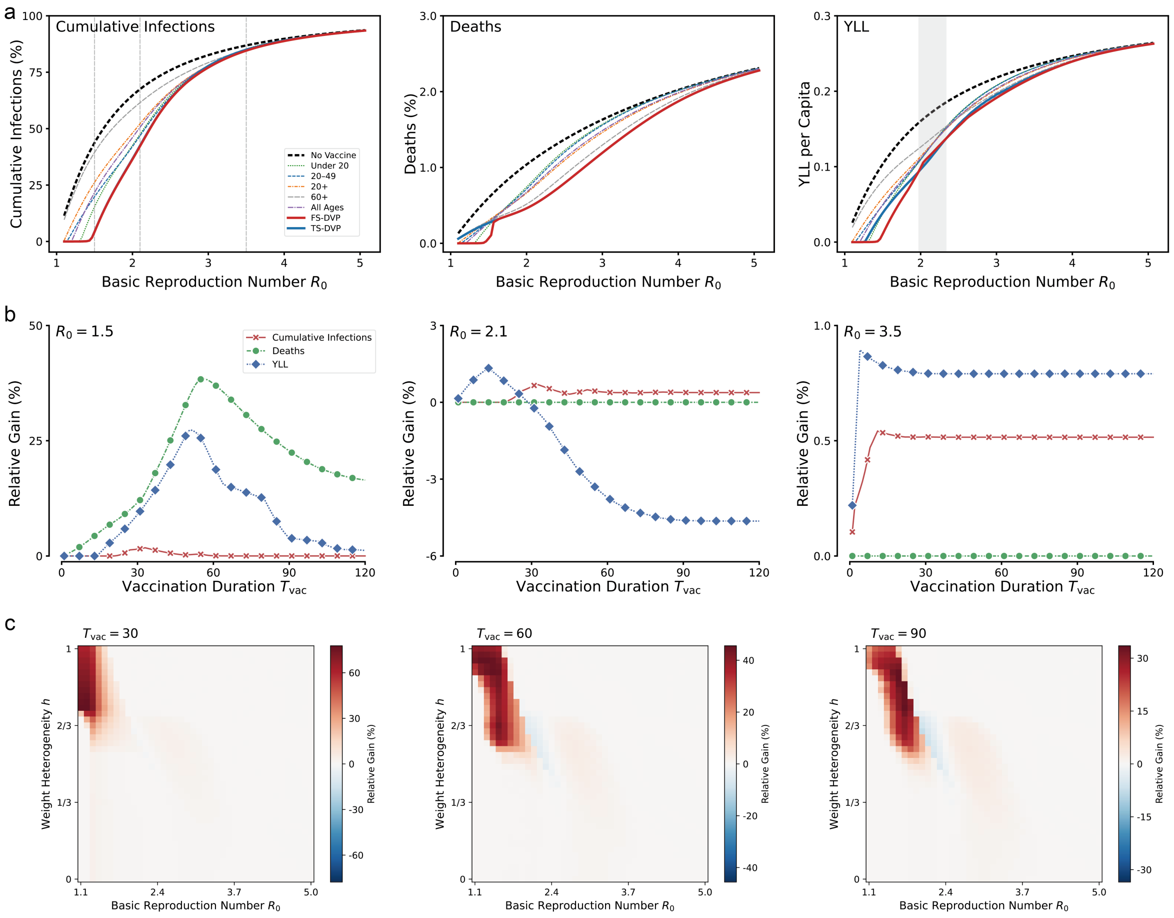


**Figure S2:** **a** Final-state cumulative infections, deaths, and years of life lost (YLL) for different vaccine allocation strategies as a function of the basic reproduction number ($R_0$). In the cumulative infections panel, vertical dashed lines indicate $R_0 = 1.5$, 2.1, and 3.5, which are the parameter settings analyzed in panels (b) and (c). In the YLL panel, the gray shaded region marks the interval $R_0 \in [1.98, 2.36]$, where FS-DVP does not yield the best performance, highlighting an exception to its overall superiority. **b** Relative gain (%) of FS-DVP over TS-DVP for reducing cumulative infections, deaths, and YLL, plotted against vaccination campaign duration ($T_{\text{vac}}$), shown separately for $R_0 = 1.5$, 2.1, and 3.5. **c** Joint effect of transmission and objective-weight heterogeneity: heatmaps show the relative gain (in %) across $(R_0, h)$ at $T_{\text{vac}} \in \{30, 60, 90\}$ days. Red (blue) indicates that FS-DVP outperforms (underperforms) TS-DVP.

time, given the information and forecast available then. However, the concatenation of these stage-wise optimal decisions forms only a local plan for the full-horizon problem and is not guaranteed to be globally optimal, especially when the campaign spans many decision times. Small stage-wise deviations can accumulate over iterations, a standard tradeoff in model predictive control [1]. Consequently, in narrow parameter bands such as prolonged campaigns at intermediate $R_0$, the transient-state approach can occasionally attain slightly better overall outcomes.

To further assess the relative gains, we define the relative gain of FS-DVP over TS-DVP, normalized by the no-vaccination final-state burden:

$$\varpi_{\bullet} = \frac{\tilde{\chi}_{\bullet}^{\text{ts}} - \tilde{\chi}_{\bullet}^{\text{fs}}}{\tilde{\chi}_{\bullet}^{\text{non}}} \tag{S5.16}$$

where $\bullet \in \{\text{c}, \text{d}, \text{y}\}$ indexes the objective (cumulative infections, deaths, YLL). Here $\tilde{\chi}_{\bullet}^{\text{fs}}$, $\tilde{\chi}_{\bullet}^{\text{ts}}$, and $\tilde{\chi}_{\bullet}^{\text{non}}$ denote the final-state burdens under FS-DVP, TS-DVP, and no vaccination, respectively. A value $\varpi\bullet = 0$ indicates equal performance; $\varpi_{\bullet} > 0$ ($< 0$) indicates that FS-DVP is more (less) effective than TS-DVP.

Fig. S2b illustrates the relative gain of FS-DVP over TS-DVP as a function of vaccination campaign duration ($T_{\text{vac}}$) at different values of $R_0$. When $R_0 = 1.5$, FS-DVP consistently delivers positive relative gains across all objectives, with the most pronounced advantage observed for minimizing deaths. The

relative gain generally increases with longer campaign durations, reaching a maximum at intermediate durations before declining as $T_{\text{vac}}$ becomes very large. As $R_0$ increases to 2.1, FS-DVP retains a positive relative gain for cumulative infections. For deaths, however, the gain diminishes, while for YLL it is initially positive but can turn negative at longer campaign durations, indicating that TS-DVP can occasionally outperform FS-DVP in these scenarios. At $R_0 = 3.5$, the advantage of FS-DVP becomes apparent again for cumulative infections and YLL, but remains limited for deaths.

For minimizing YLL, FS-DVP can sometimes perform slightly worse than TS-DVP, because YLL optimization typically entails stronger cross-group trade-offs. When optimizing different objectives, we assign different weights across population groups: equal weights for cumulative infections, age-specific IFRs for deaths, and per-capita YLL for YLL. This implies that weight heterogeneity is smallest for cumulative infections and largest for deaths. In practice, however, YLL often generates the strongest cross-group trade-offs, because the groups that dominate transmission and those that contribute most to YLL only partially overlap. As a result, the allocation must balance indirect blocking of transmission into middle and older ages with direct protection of higher-weight groups.

To further explore this effect, we constructed a family of synthetic IFR vectors based on the empirically derived age-stratified IFRs. Specifically,

$$\boldsymbol{\epsilon}_h = (\boldsymbol{\epsilon} - \bar{\epsilon}\mathbf{1})h + \bar{\epsilon}\mathbf{1} \tag{S5.17}$$

where $\bar{\epsilon}$ is the mean of all elements of $\boldsymbol{\epsilon}$. The parameter $h$ adjusts the heterogeneity of the weight distribution, referred to as weight heterogeneity. When $h = 0$, $\boldsymbol{\epsilon}_h$reduces to a homogeneous vector with zero heterogeneity; when $h = 1$, $\boldsymbol{\epsilon}_h$ecovers the original IFRs. Increasing $h$ produces greater heterogeneity. Using $\boldsymbol{\epsilon}_h$ as the IFRs, we simulated epidemic dynamics under FS-DVP, TS-DVP, and a no-vaccination baseline. As shown in Fig. S2c, we evaluated, at three values of $T_{\text{vac}}$, how weight heterogeneity $h$ and $R_0$ jointly modulate the relative gain for reducing deaths. We find that when both the weight heterogeneity and $R_0$ are in a moderate range, TS-DVP can slightly outperform FS-DVP, precisely the region where trade-offs across groups are strongest.

Mechanistically, when $R_0$ is low, indirect protection is strong and vaccinating high-contact groups ultimately benefits high-importance groups; FS-DVP captures this long-horizon effect and dominates. When $R_0$ is high, blocking becomes ineffective and both strategies converge to direct protection, so the difference shrinks. At intermediate $R_0$ with moderate heterogeneity, the marginal vaccination benefits across groups become similar and nearly parallel, so FS-DVP spreads doses to preserve long-term benefits, whereas TS-DVP concentrates on high-importance groups to secure immediate direct benefits. Over many decision rounds, small receding-horizon deviations can accumulate for FS-DVP and, in this strong-trade-off regime, can translate into a slight disadvantage, most visibly for YLL. These phenomenon also suggests that no single strategy is always superior under all conditions.

# Supplementary Note 6 Mechanistic Insights with Distinct Optimization Objectives

We further investigate the mechanistic insights on time-varying optimal vaccine prioritization under different optimization objectives in Fig. S3. Throughout this analysis we set $R_0 = 2$ and the daily vaccine supply to $\theta = 0.35\%$, with empirical strategies for reference.

The optimal vaccine allocation schedules differ substantially depending on the optimization objective. As illustrated in Fig. S3a–f, when minimizing cumulative infections, the strategy initially allocates all vaccines to the 10–19 age group, then gradually shifts portions of the supply to the 30–39, 20–29, 40–49, and finally 0–9 age groups. For minimizing deaths, vaccines are first entirely allocated to the 70+ group, then sequentially switched in full to the 60–69, 50–59, and 40–49 age groups. In contrast, when minimizing YLL, the strategy prioritizes the 50–59 age group initially, then fully switches to the 10–19

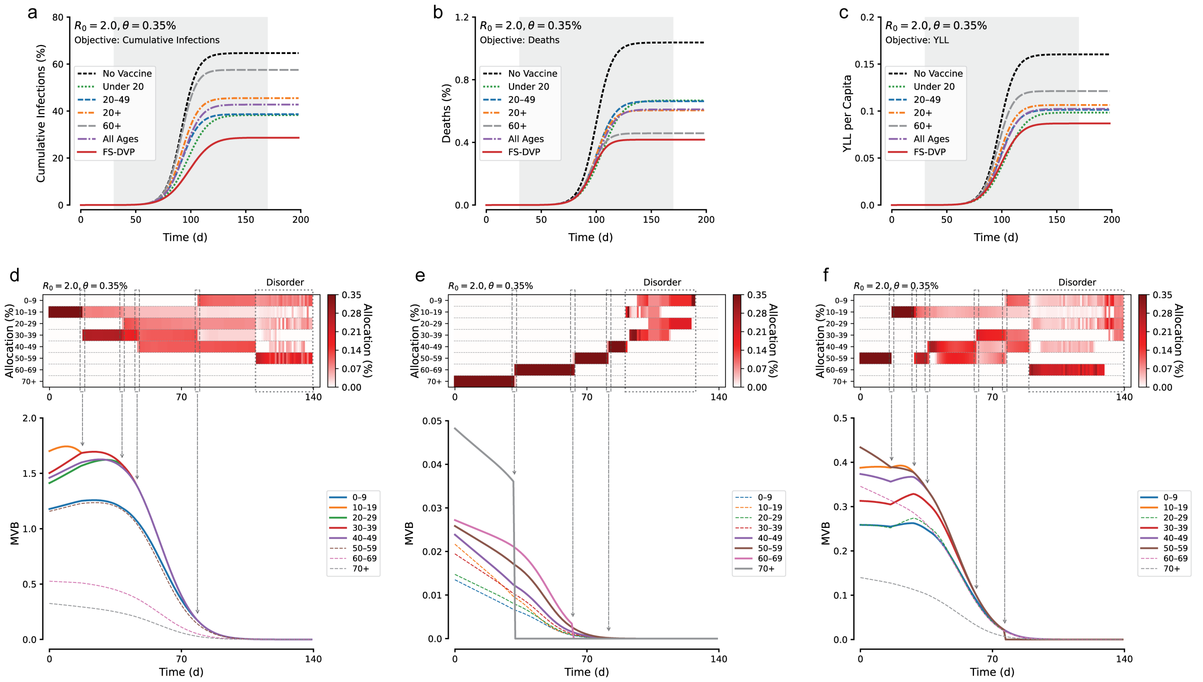


**Figure S3:** **a**–**c** Time courses of cumulative infected fraction (a), death fraction (b), and YLL per capita (c) under different strategies at $R_0 = 2.0$. The daily vaccine supply is $\theta = 0.35\%$ of the population. The gray band marks the 140-day vaccination period. **d**–**f** Top subpanels: time-varying optimal allocations produced by our method; dashed rectangles mark switching times. The dotted band highlights the late-campaign disorder where optimization potential is low. Bottom subpanels: MVB $\xi_l$ for each age group $l$ over time; arrows indicate where the leading MVB curves align with allocation switches, merging for the cumulative-infections and YLL objectives (**d** and **f**) and intersecting for the deaths objective (textbfe).

group, and subsequently distributes vaccines in parts to the 50–59, 40–49, 30–39, and 0–9 age groups. Each partial reallocation corresponds to a merging of the leading MVB curves (MVB merge), while each complete reallocation corresponds to an intersection of MVB curves (MVB intersection).

It is evident that both the dynamic allocation patterns and the switching mechanisms change depending on the optimization objective. For example, when minimizing deaths, the MVB for the prioritized elderly age group (e.g., 70+) drops sharply to zero as soon as all susceptible individuals in that group are vaccinated, leading to a MVB intersection and a complete reallocation of vaccines. In general, the MVB for a given age group becomes zero only under two conditions: when there are no remaining susceptibles in that group, or when the epidemic has reached its final state. Prior to the end of the epidemic, even a single susceptible individual in a group can yield a high MVB; however, as soon as the susceptible count drops to zero, the MVB instantaneously vanishes. This is because MVB fundamentally measures the marginal impact of each susceptible individual within an age group on the final state, rather than the effect of the entire group as a whole. Even if only one susceptible remains in that age group, that person can still interact with other age groups, potentially initiating new chains of transmission and influencing the ultimate course of the epidemic. This phenomenon is also observed in the YLL-minimization scenario, for example, during the fifth allocation switch when the 50–59 group's susceptibles are exhausted and their MVB drops to zero.

For different optimization objectives, the weighting assigned to each age group within the optimization framework varies accordingly, which in turn leads to distinct vaccine allocation strategies: all age groups are weighted equally for minimizing cumulative infections; for deaths, weights are proportional to IFRs; and for YLL, weights reflect the per-capita YLL. Thus, when minimizing deaths, the elderly receive the highest weight and thus the highest initial MVB, causing the strategy to fully allocate vaccines to them first. Once their susceptibles are depleted, the MVB drops sharply to zero, resulting in a complete switch

in vaccine allocation to the next most impactful age group.

## Supplementary Note 7 Mathematical Explanation for Merging and Intersection of MVB Curves

The phenomenon of MVB merging and intersection during optimal allocation can be rigorously explained through the lens of constrained optimization. At each decision time, the vaccine allocation vector $\boldsymbol{\vartheta}_t = [\vartheta_{1;t}, \vartheta_{2;t}, ..., \vartheta_{n;t}]^\mathsf{T}$ across $n$ population groups is determined by minimizing the cost function (e.g., predicted final-state cumulative infections, deaths, or YLL), subject to constraints such as the total vaccine supply $\sum_{l=1}^{n} \vartheta_{l;t}\rho_l = \theta$ and non-negativity $0 \leq \vartheta_{l;t} \leq s_l(t)$. The MVB for group $l$ is defined as the negative partial derivative of the objective with respect to $\vartheta_l$ at the optimum, as in Eqs. (13)–(15) in the main text. Here, $\xi_{l;t}$ refers to the MVB associated with minimizing cumulative infections ($\xi^{\mathrm{c}}_{l;t}$), deaths ($\xi^{\mathrm{d}}_{l;t}$), or YLL ($\xi^{\mathrm{y}}_{l;t}$), depending on the selected objective, for age group $l$ at time $t$.

A merge occurs when the optimizer allocates nonzero doses to multiple competing groups (e.g., groups $l$ and $m$), and the Karush-Kuhn-Tucker (KKT) first-order optimality conditions require that the Lagrange multipliers associated with the equality and inequality constraints are such that [2]

$$\xi_{l;t} = \xi_{m;t} = \lambda \tag{S7.18}$$

where $\lambda$ is the Lagrange multiplier for the total vaccine constraint. This means the MVB of allocating additional vaccine to these groups is equal, and no infinitesimal reallocation between them can further reduce the objective. Geometrically, the solution lies on a "face" of the feasible region where the gradients (MVBs) for the active groups are equal and aligned with the constraint hyperplane.

An intersection corresponds to the optimizer reaching a "corner" or boundary of the feasible region, specifically, allocating all available vaccine to a single group (e.g., group $l$), while other groups receive zero. Here,

$$\xi_{l;t} = \lambda > \xi_{m;t}, \quad \forall m \neq l \tag{S7.19}$$

That is, group $l$ has a strictly higher marginal benefit than all other groups, so the optimal strategy is to allocate all doses to $l$ until the MVBs cross (intersect), at which point the allocation shifts abruptly to another group whose MVB becomes dominant.

Thus, the merging of MVB curves reflects situations where the optimal solution involves shared allocation (multiple nonzero $\vartheta_{l;t}$) with equal marginal utility, while intersection reflects a shift in the active constraint, resulting in abrupt changes in allocation. These are direct consequences of the necessary optimality conditions in constrained, time-varying epidemic control problems.

In practice, the SLSQP algorithm used in our study approximates these KKT conditions numerically at each optimization step, supporting the theoretical basis for interpreting observed MVB merging and intersection phenomena.

## Supplementary Note 8 Coarse-Grained Approximations of Dynamic Vaccine Prioritization

FS-DVP adjusts the vaccine mix almost daily. While this fine-grained reallocation is effective, it can substantially increase implementation costs in practice due to frequent updates, communication, and logistics. To ease this burden without sacrificing performance, we construct coarse-grained schedules that update only at a few key time points.

We first identify the switching points in the dynamic schedule, i.e., times when the priority ordering implied by the policy changes, and use them to divide the vaccination horizon into a small number

of discrete intervals. Within each interval, instead of following the day-to-day FS-DVP updates, we implement a single constant allocation equal to the average FS-DVP allocation over that interval. This yields a stepwise schedule that preserves the overall structure of FS-DVP but is far easier to implement, which we refer to as the Piecewise-constant strategy.

Starting from the Piecewise-constant strategy as an initial candidate, we then apply an optimization algorithm to fine-tune the allocation proportions within each interval while keeping the switching points fixed. The adjustments are chosen to minimize the final-state burden, by forward simulating the vaccination process and then using our final-state predictor to estimate the outcomes. This procedure effectively warm-starts a new optimization process from the Piecewise-constant strategy, which is already close to optimal, thereby greatly reducing the number of iterations required. The result is an Optimized Piecewise-constant strategy.

Fig. S4 compares FS-DVP, the Piecewise-constant strategy, the optimized Piecewise-constant strategy, and no vaccination. Fig. S4a shows that both the Piecewise-constant and Optimized Piecewise-constant strategies closely track the epidemic trajectory of FS-DVP and substantially reduce cumulative infections relative to no vaccination. Fig. S4b–d display the corresponding allocation sequences. Compared with the rapidly varying FS-DVP schedule, the Piecewise-constant and optimized Piecewise-constant schedules change only at a few switching points, making them far more stable and easier to implement. In this scenario, the optimized piecewise-constant strategy provides no additional measurable gains, indicating that coarse-graining preserves the effectiveness of FS-DVP while greatly reducing operational complexity.

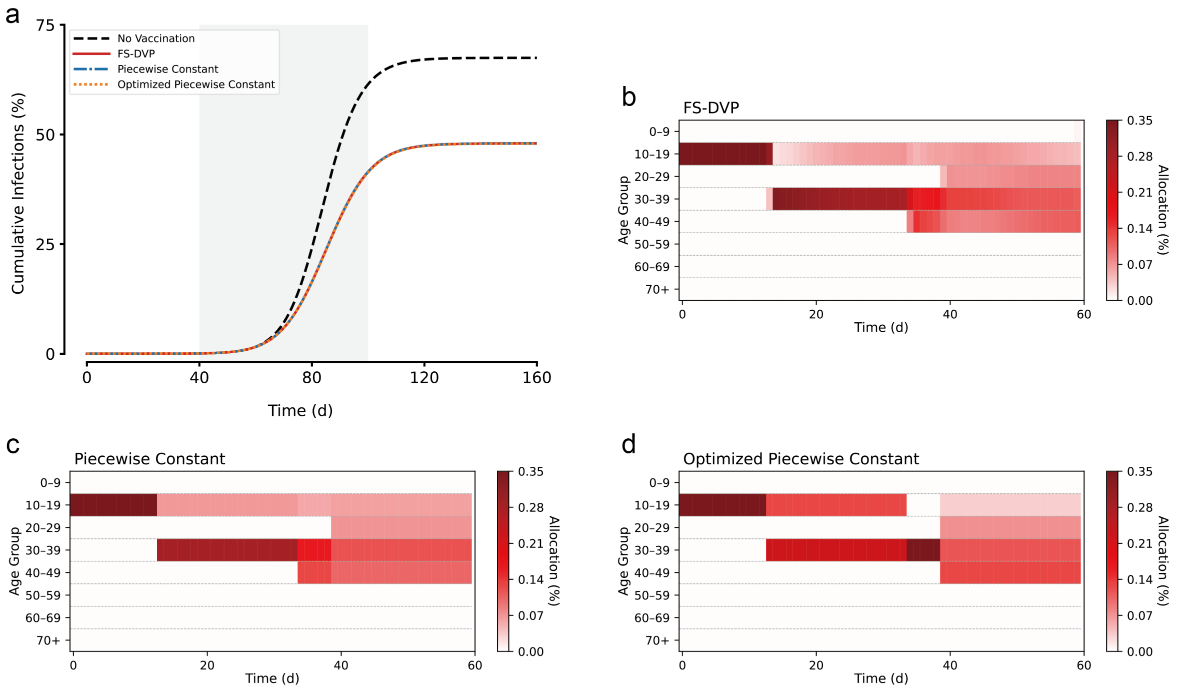


**Figure S4:** Coarse-graining a dynamic vaccination policy into piecewise-constant schedules. **a** Cumulative infections under four policies: No Vaccination (black dashed), FS-DVP (solid), Piecewise-constant (dash-dotted), and Optimized Piecewise-constant (dotted). The grey shading marks the vaccination window. Both Piecewise-constant and Optimized Piecewise-constant schedules closely track FS-DVP and substantially outperform No Vaccination. **b**–**d** Allocation sequences (fraction of doses by age group) for FS-DVP (**b**), Piecewise-constant (**c**), and Optimized Piecewise-constant (**d**). Switching points are detected from changes in FS-DVP's priority ordering and define the piecewise intervals. The Piecewise-constant strategy assigns a single fixed allocation within each interval, while the Optimized Piecewise-constant strategy refines these per-interval proportions using the final-state predictor. Both variants yield stable, operationally simple schedules that maintain FS-DVP-level performance.

# Supplementary Note 9 Population Distribution

For each country included in this study, we obtain age-stratified population distributions from Ref. [3] (Supplementary Fig. S5). Each country's population is divided into eight age groups: 0–9, 10–19, 20–29, 30–39, 40–49, 50–59, 60–69, and 70+ years. The resulting distributions are used as input parameters for the age-structured epidemic model, ensuring that simulated transmission and vaccination dynamics accurately reflect country-specific demographic structures. For some countries, the proportion of individuals aged 70 years and above is particularly high, both because of the severity of population aging in these countries and because we classify all individuals aged 70 years and over into a single group rather than using 10-year intervals as for younger age groups.

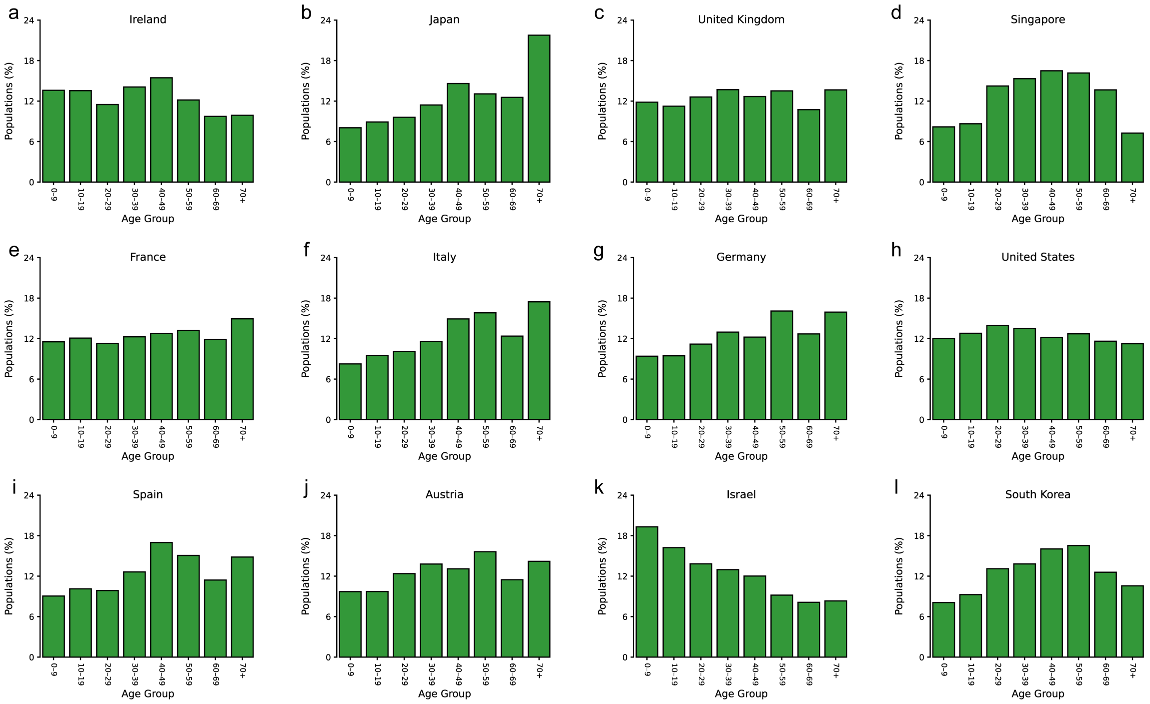


**Figure S5:** Age-stratified population distributions for twelve countries. Bar plots show the percentage of the total population in each age group for (**a**) Ireland, (**b**) Japan, (**c**) United Kingdom, (**d**) Singapore, (**e**) France, (**f**) Italy, (**g**) Germany, (**h**) United States, (**i**) Spain, (**j**) Austria, (**k**) Israel, and (**l**) South Korea. Population structures are obtained from official national census sources or publicly available datasets. These distributions provide the demographic basis for all age-stratified modeling and optimization analyses in this study.

Across the twelve countries examined, population age structures display clear heterogeneity (Supplementary Fig. S5). Notably, Japan and Italy exhibit pronounced population aging, with a substantial proportion of individuals in the 60–69 and 70+ age groups. In contrast, countries such as Israel and Singapore show comparatively larger fractions in younger age brackets, reflecting higher birth rates and/or different demographic histories. Several European countries, including Ireland, France, and the United Kingdom, have relatively balanced distributions across age groups, but still show an increasing proportion in older age brackets due to population aging trends. These differences in demographic structure critically shape epidemic dynamics and the optimal allocation of vaccines, as age-related susceptibility, transmission, and severity profiles interact with population composition.

# Supplementary Note 10 Contact Matrix

Age-stratified contact matrices are extracted from Prem et al. [4], which provides synthetic contact estimates for 152 countries based on demographic and survey data (Supplementary Fig. S6). Each entry

reflects the average normalized number of contacts per person per day between age groups. The matrices were used to specify transmission patterns in the age-structured model.

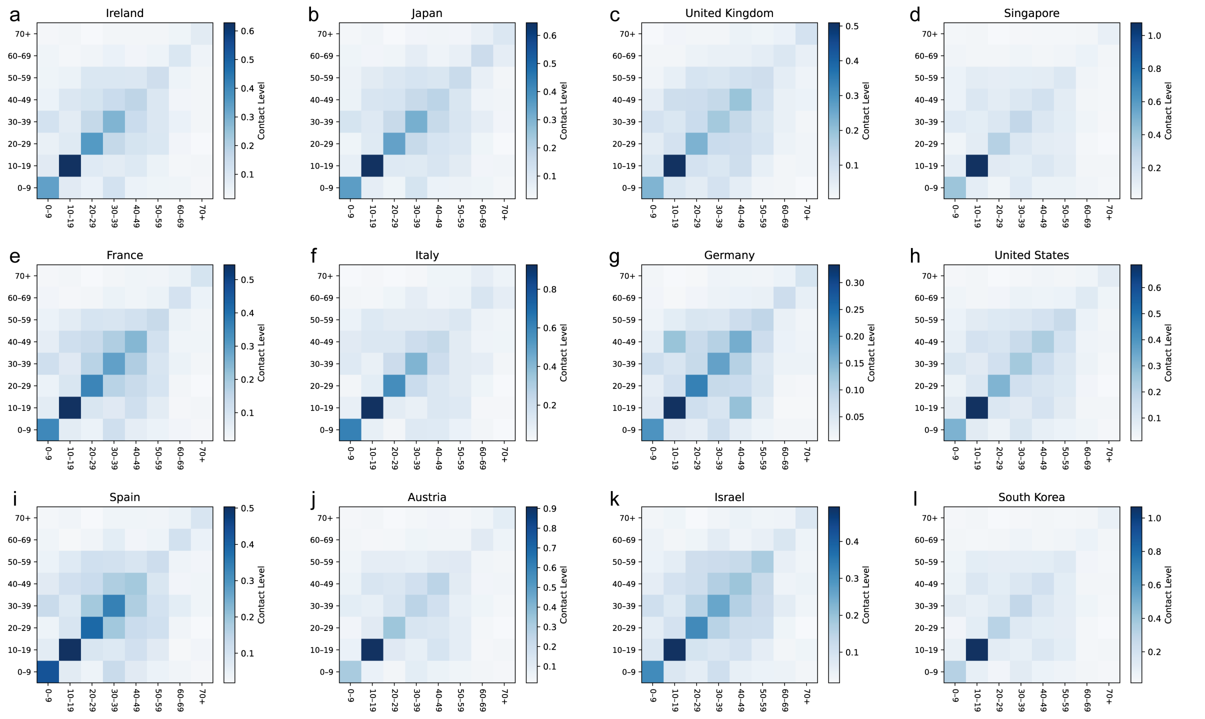


**Figure S6:** Heatmaps illustrate contact intensities between different age groups for (**a**) Ireland, (**b**) Japan, (**c**) United Kingdom, (**d**) Singapore, (**e**) France, (**f**) Italy, (**g**) Germany, (**h**) United States, (**i**) Spain, (**j**) Austria, (**k**) Israel, and (**l**) South Korea. Color intensity indicates the relative frequency of contacts between age groups, as estimated from national or international contact surveys. These matrices underlie the age-structured transmission dynamics modeled in the main text.

The empirical contact matrices reveal differences in age-mixing patterns across countries (Supplementary Fig. S6). Most countries display a strong diagonal, indicating that individuals predominantly interact with others within their own age group. In addition, significant off-diagonal contacts are observed between younger and middle-aged groups, reflecting school, workplace, and intergenerational household mixing. For example, Singapore and Israel have especially pronounced within-child and within-young-adult contacts, consistent with their larger youth populations and household structures. European countries typically show more evenly distributed contact intensities among adults and elderly, indicative of diverse social mixing patterns. These contact matrix structures play a pivotal role in shaping epidemic spread and modulate the impact of age-targeted vaccination strategies.

# Supplementary Note 11 Infection Fatality Rates

We adopt age-stratified IFRs from Ref. [5] (Spanish sero-epidemiological study). As shown in Supplementary Fig. S7, the IFRs increases dramatically with age, from below 0.1% for individuals under 40 to approximately 5% for those aged 60–69, and exceeding 18% for those 70 and older. This pattern, confirmed by Ref. [5], is remarkably consistent across diverse national settings and forms the basis for our calculations of age-stratified mortality and years of life lost (YLL) in the model. These values are robust across multiple countries and support the generalizability of our results regarding optimal vaccine prioritization.

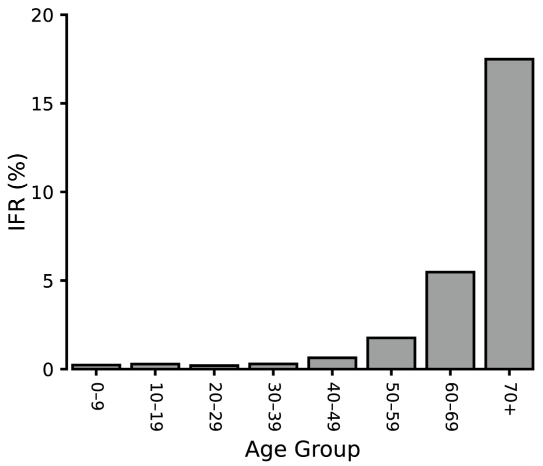


**Figure S7:** Age-stratified infection fatality rates (IFRs) used in our analysis. The IFR increases sharply with age, rising from less than 0.1% in the youngest age groups to over 18% in the 70+ group. These values are based on the estimates from Ref. [5], which show a consistent pattern across different countries.

# Supplementary Note 12 Years of Life Lost

The age-stratified per-capita years of life lost (YLL) shown here is estimated for each country by multiplying the IFRs of each age group by their remaining life expectancy, based on national demographic data. This measure captures the direct impact of a COVID-19 infection in terms of YLL for each age group. The pattern is similar in all countries: older adults face a much higher per-capita YLL risk than younger groups, due to both higher IFR and remaining life expectancy. This highlights why prioritizing vaccination among high-risk older age groups can have a large impact on reducing the overall burden of YLL. Age-stratified IFR values are taken from Ref. [5], and life expectancy are sourced from the WHO's data [6].

# References


[1] Mayne, D. Q., Rawlings, J. B., Rao, C. V. & Scokaert, P. O. Constrained model predictive control: Stability and optimality. *Automatica* **36**, 789–814 (2000).

[2] Kuhn, H. W. & Tucker, A. W. Nonlinear programming. In *Traces and emergence of nonlinear programming*, 247–258 (Springer, 2013).

[3] United nations, "world population prospects 2019". `https://population.un.org/wpp/` (Accessed 29 June 2021).

[4] Prem, K., Cook, A. R. & Jit, M. Projecting social contact matrices in 152 countries using contact surveys and demographic data. *PLoS Computational Biology* **13**, e1005697 (2017).

[5] Centro de coordinacion de alertas y emergencias sanitarias, "actualizacion n 103. enfermedad por el coronavirus (covid-19). 12.05.2020". `https://www.mscbs.gob.es/profesionales/saludPublica/ccayes/alertasActual/nCov/documentos/Actualizacion_103_COVID-19.pdf` (Accessed 29 June 2021).

[6] World health organization, "life expectancy and healthy life expectancy, data by country". `https://apps.who.int/gho/data/node.main.688` (Accessed 29 June 2021).

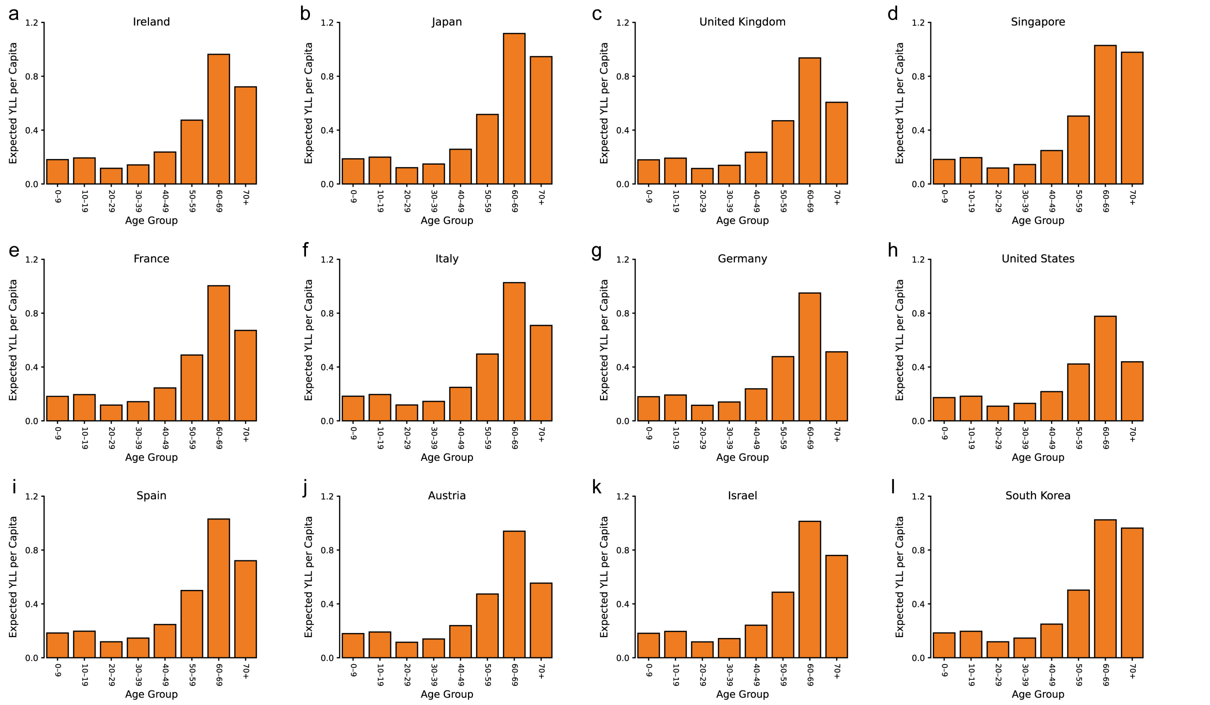


**Figure S8:** Age-stratified per-capita years of life lost (YLL) from infection for (**a**) Ireland, (**b**) Japan, (**c**) United Kingdom, (**d**) Singapore, (**e**) France, (**f**) Italy, (**g**) Germany, (**h**) United States, (**i**) Spain, (**j**) Austria, (**k**) Israel, and (**l**) South Korea. For each age group, this metric is calculated as the product of that group's infection fatality rate (IFRs) and their average remaining life expectancy, using national demographic and IFR data. The result reflects the direct risk of infection to each age group, with older cohorts facing much higher YLL per infection due to elevated fatality risk and remaining life years.
